# Supplementary material for: WELL: Applying Bug Detectors to Bug Localization via Weakly Supervised Learning
Source: arXiv:2305.17384 source file (2023-06-08)
Supplement: Supplementary file 1 [file hasNext11.tex]

\begin{CJK*}{UTF8}{gbsn}\scriptsize
{\setlength{\fboxsep}{0pt}\colorbox{white!0}{\parbox{0.9\textwidth}{
\colorbox{black!1.4569694}{\strut public} \colorbox{black!1.2766428}{\strut boolean} \colorbox{black!37.7141}{\strut hasNext} \colorbox{black!3.8408546}{\strut (} \colorbox{black!0.39984882}{\strut )} \colorbox{black!0.2314061}{\strut \{} \colorbox{black!4.980752}{\strut return} \colorbox{black!9.051436}{\strut count} \fcolorbox{red}{black!12.345039}{\strut $<=$} \colorbox{black!3.1659663}{\strut array} \colorbox{black!9.354168}{\strut .} \colorbox{black!9.539014}{\strut length} \colorbox{black!1.195401}{\strut ;} \colorbox{black!2.4163127}{\strut \}} 
}}}
\end{CJK*}
