# Supplementary material for: WELL: Applying Bug Detectors to Bug Localization via Weakly Supervised Learning
Source: arXiv:2305.17384 source file (2023-06-08)
Supplement: Supplementary file 2 [file hasNext2.tex]

\begin{CJK*}{UTF8}{gbsn}\scriptsize
{\setlength{\fboxsep}{0pt}\colorbox{white!0}{\parbox{0.9\textwidth}{
\colorbox{black!4.55071}{\strut public} \colorbox{black!2.424121}{\strut boolean} \colorbox{black!14.476347}{\strut hasNext} \colorbox{black!4.550567}{\strut (} \colorbox{black!4.3730855}{\strut )} \colorbox{black!0.9687662}{\strut \{} \colorbox{black!8.533886}{\strut return} \colorbox{black!11.396038}{\strut count} \fcolorbox{red}{black!2.1994889}{\strut $<=$} \colorbox{black!13.802833}{\strut array} \colorbox{black!8.497029}{\strut .} \colorbox{black!7.395506}{\strut length} \colorbox{black!3.6109269}{\strut ;} \colorbox{black!3.9337456}{\strut \}} 
}}}
\end{CJK*}
