# Supplementary material for: WELL: Applying Bug Detectors to Bug Localization via Weakly Supervised Learning
Source: arXiv:2305.17384 source file (2023-06-08)
Supplement: Supplementary file 3 [file hasNext7.tex]

\begin{CJK*}{UTF8}{gbsn}\scriptsize
{\setlength{\fboxsep}{0pt}\colorbox{white!0}{\parbox{0.9\textwidth}{
\colorbox{black!0.077456236}{\strut public} \colorbox{black!0.027169287}{\strut boolean} \colorbox{black!10.271729}{\strut hasNext} \colorbox{black!0.3438279}{\strut (} \colorbox{black!0.019343197}{\strut )} \colorbox{black!0.004684925}{\strut \{} \colorbox{black!0.05212426}{\strut return} \colorbox{black!13.807848}{\strut count} \fcolorbox{red}{black!51.454807}{\strut $<=$} \colorbox{black!1.8669128}{\strut array} \colorbox{black!0.852561}{\strut .} \colorbox{black!0.5052209}{\strut length} \colorbox{black!0.10697842}{\strut ;} \colorbox{black!0.010097027}{\strut \}} 
}}}
\end{CJK*}
